# Supplementary material for: Generative Models for Novelty Detection: Applications in abnormal event and situational change detection from data series
Source: arXiv:1904.04741 source file (2019-04-09)
Supplement: Supplementary file 2 [file appendix2.tex]

%!TEX root = ../thesis.tex
% ******************************* Thesis Appendix B ********************************

\chapter{Installing the CUED class file}

\LaTeX.cls files can be accessed system-wide when they are placed in the
<texmf>/tex/latex directory, where <texmf> is the root directory of the user’s \TeX installation. On systems that have a local texmf tree (<texmflocal>), which
may be named ``texmf-local'' or ``localtexmf'', it may be advisable to install packages in <texmflocal>, rather than <texmf> as the contents of the former, unlike that of the latter, are preserved after the \LaTeX system is reinstalled and/or upgraded.

It is recommended that the user create a subdirectory <texmf>/tex/latex/CUED for all CUED related \LaTeX class and package files. On some \LaTeX systems, the directory look-up tables will need to be refreshed after making additions or deletions to the system files. For \TeX Live systems this is accomplished via executing ``texhash'' as root. MIK\TeX users can run ``initexmf -u'' to accomplish the same thing.

Users not willing or able to install the files system-wide can install them in their personal directories, but will then have to provide the path (full or relative) in addition to the filename when referring to them in \LaTeX.
