# Supplementary material for: Generative Models for Novelty Detection: Applications in abnormal event and situational change detection from data series
Source: arXiv:1904.04741 source file (2019-04-09)
Supplement: Supplementary file 3 [file cover_back.tex]

%!TEX root = ../thesis.tex
% ******************************* Thesis Appendix A ****************************
Novelty detection is a process for distinguishing the observations that differ in some respect from the observations that a model is trained on. This set of observations that are extremely deviated from other observations called Outliers. Usually, outliers are not noise, they can be seen as a source of information that may represent a different class (generating mechanism) of data. There vast number of applications are designed based on outliers detection (e.g., fraud detection, medicine, surveillance, continual learning). The core of all these applications is a set of one-class classifiers and generative methods which can efficiently model such problems. In this thesis, we focused on the two main applications of novelty detection: abnormality detection in the crowded scenes for surveillance applications, and situational change detection for continual learning in autonomous agents. We propose several methods to model the novelty detection problem in unsupervised and semi-supervised fashion.
